# Supplementary material for: Real-Time Refocusing using an FPGA-based Standard Plenoptic Camera
Source: arXiv:2010.07746 source file (2020-10-09)
Supplement: Supplementary file 1 [file suppl_VHDL_code_pub.pdf]

## APPENDIX

```

1  -----
2  -- Company:      Brunel University, Uxbridge, Greater London, UK
3  -- Engineer:     Christopher Hahne
4  --
5  -- Create Date:  17:24:10 03/08/2013
6  -- Module Name:  shift_and_integration - Behavioral
7  -- Description:   MWE for 5 pixel micro image resolution
8  -----
9  library IEEE;
10 use IEEE.STD_LOGIC_1164.ALL;
11 use IEEE.NUMERIC_STD.ALL;
12
13 entity shift_and_integration is
14   generic(
15     D : integer := 3; -- colour channels
16     S : integer := 8; -- pixel bit depth
17     M : integer := 5 -- one-dimensional micro image resolution
18   );
19   port(
20     PCLKx2      : in  STD_LOGIC;
21     RST         : in  STD_LOGIC;
22     btn_up      : in  STD_LOGIC;
23     btn_down    : in  STD_LOGIC;
24     rgb_w       : out STD_LOGIC_VECTOR(23 downto 0) := (others => '0');
25     rgb_r       : in  STD_LOGIC_VECTOR(23 downto 0);
26     hCounter    : in  UNSIGNED(10 downto 0);
27     vCounter    : in  UNSIGNED(9  downto 0);
28     bs_done     : in  STD_LOGIC
29   );
30 end shift_and_integration;
31
32 architecture Behavioral of shift_and_integration is
33
34   constant shift_max : integer := (M**2)-1;
35
36   signal gear : STD_LOGIC := '0';
37   signal shift : UNSIGNED(5 downto 0) := "000001"; -- default
38   signal new_shift : UNSIGNED(5 downto 0) := (others => '0');
39   signal fraction : STD_LOGIC_VECTOR((D*S)-1 downto 0) := (others => '0');
40   signal reg_E : STD_LOGIC_VECTOR((D*S)-1 downto 0) := (others => '0');
41   signal reg_D : STD_LOGIC_VECTOR((D*S)-1 downto 0) := (others => '0');
42   signal reg_C : STD_LOGIC_VECTOR((D*S)-1 downto 0) := (others => '0');
43   signal reg_B : STD_LOGIC_VECTOR((D*S)-1 downto 0) := (others => '0');
44   signal reg_A : STD_LOGIC_VECTOR((D*S)-1 downto 0) := (others => '0');
45   signal count : UNSIGNED(3 downto 0) := (others => '0');
46
47 begin
48
49   -- replicate shift and integrate process for D colour channels
50   loop0 : for i in 1 to D generate
51     process(PCLKx2, RST, gear, shift, fraction)
52     begin
53       if rising_edge(PCLKx2) then
54         if RST = '1' then -- or blank_in = '1' then
55           reg_E((i*S-1) downto ((i-1)*S)) <= (others => '0');
56           reg_D((i*S-1) downto ((i-1)*S)) <= (others => '0');
57           reg_C((i*S-1) downto ((i-1)*S)) <= (others => '0');
58           reg_B((i*S-1) downto ((i-1)*S)) <= (others => '0');
59           reg_A((i*S-1) downto ((i-1)*S)) <= (others => '0');
60         elsif gear = '1' then
61           case shift is
62             when "000001" =>
63               reg_E((i*S-1) downto ((i-1)*S)) <= fraction((i*S-1) downto ((i-1)*S));
64               reg_D((i*S-1) downto ((i-1)*S)) <= std_logic_vector(unsigned(reg_D((i*S-1) downto ((i-1)*S)))
65                 + unsigned(fraction((i*S-1) downto ((i-1)*S))));
66               reg_C((i*S-1) downto ((i-1)*S)) <= std_logic_vector(unsigned(reg_C((i*S-1) downto ((i-1)*S)))
67                 + unsigned(fraction((i*S-1) downto ((i-1)*S))));
68               reg_B((i*S-1) downto ((i-1)*S)) <= std_logic_vector(unsigned(reg_B((i*S-1) downto ((i-1)*S)))
69                 + unsigned(fraction((i*S-1) downto ((i-1)*S))));
70               reg_A((i*S-1) downto ((i-1)*S)) <= std_logic_vector(unsigned(reg_A((i*S-1) downto ((i-1)*S)))
71                 + unsigned(fraction((i*S-1) downto ((i-1)*S))));
72               rgb_w((i*S-1) downto ((i-1)*S)) <= std_logic_vector(unsigned(reg_A((i*S-1) downto ((i-1)*S)))
73                 + unsigned(fraction((i*S-1) downto ((i-1)*S))));
74             when others =>
75               null;
76           end case;
77         end if;
78       end if;
79     end process;
80   end loop;
81
82 end Behavioral;

```

```

71     end case;
72 else
73     reg_E((i*S-1) downto ((i-1)*S)) <= (others => '0');
74     reg_D((i*S-1) downto ((i-1)*S)) <= reg_E((i*S-1) downto ((i-1)*S));
75     reg_C((i*S-1) downto ((i-1)*S)) <= reg_D((i*S-1) downto ((i-1)*S));
76     reg_B((i*S-1) downto ((i-1)*S)) <= reg_C((i*S-1) downto ((i-1)*S));
77     reg_A((i*S-1) downto ((i-1)*S)) <= reg_B((i*S-1) downto ((i-1)*S));
78 end if;
79 end if;
80 end process;
81
82 -- ROM based divider
83 ROM_divider: entity work.blk_mem_gen_v6_2 PORT MAP (
84     clka => PCLKx2,
85     ena => gear,
86     addra => rgb_r((i*S-1) downto ((i-1)*S)),
87     douta => fraction((i*S-1) downto ((i-1)*S))
88 );
89
90 end generate ;
91
92 -- gear generation
93 process(PCLKx2, bs_done, RST)
94 begin
95     if rising_edge(PCLKx2) then
96         if RST = '1' then
97             gear <= '0';
98         elsif bs_done = '1' then
99             if gear = '1' then
100                 gear <= '0';
101                 if count = (M*2)-1 then
102                     count <= (others => '0');
103                 else
104                     count <= count + 1;
105                 end if;
106             else
107                 gear <= '1';
108             end if;
109         end if;
110     end if;
111 end process;
112
113 -- shift handling
114 process(PCLKx2, btn_up, btn_down, hCounter)
115 begin
116     if rising_edge(PCLKx2) then
117         if btn_up = '1' and shift < shift_max then
118             new_shift <= shift + 1;
119         elsif btn_down = '1' and shift > "000000" then
120             new_shift <= shift - 1;
121         end if;
122         -- update only when in vertical synchronisation
123         if hCounter > 720 then
124             shift <= new_shift;
125         end if;
126     end if;
127 end process;
128
129 end Behavioral;

```
